# Supplementary material for: Toffee: Efficient Million-Scale Dataset Construction for Subject-Driven Text-to-Image Generation
Source: arXiv:2406.09305 source file (2024-08-07)
Supplement: Supplementary file 1 [file 6_appendix.tex]

% \clearpage
% \appendix
% \section{More Results}
